# Supplementary material for: Twin lead ballistic conductor based on nanoribbon edge transport
Source: arXiv:1701.03815 ancillary file (2017-10-31)
Supplement: Supplementary file 1 [file SupplemMater.pdf]

# Supplementary Material to the paper **Twin lead ballistic conductor based on nanoribbon edge transport**

Martin Konôpka* and Peter Dieška

SLOVAK UNIVERSITY OF TECHNOLOGY in Bratislava,
Faculty of Electrical Engineering and Information Technology,
Institute of Nuclear and Physical Engineering,
Department of Physics,
Ilkovičova 3, 812 19 Bratislava, Slovak Republic

*E-mail: martin.konopka@stuba.sk

31st October 2017

## 1 Eigensystems for semi-infinite chains

Consider a semi-infinite chain of identical equidistantly placed atoms. One explicit orbital $|l\rangle$ per atom at site $l$ is assumed and the independent-electron model is used. Individual lattice sites $l$ (and associated atoms and orbitals) are indexed starting from 1. The orbitals presumably form an orthonormal and complete set:

$$\langle l|l'\rangle = \delta_{ll'} \tag{1}$$

and

$$\sum_{l=1}^{\infty} |l\rangle\langle l| = \hat{1}\,. \tag{2}$$

The quantum-mechanical description of such a wire then starts with a hamiltonian of the form

$$\hat{H} = \sum_{l=1}^{\infty} \left[ \epsilon\, a_l^\dagger a_l + \sum_{m=1}^{N_{\text{far}}} t_m (a_{l+m}^\dagger a_l + a_l^\dagger a_{l+m}) \right], \tag{3}$$

where $\epsilon$ is the atomic on-site energy (same for each atom) and $t_1$, $t_2$, ..., $t_{N_{\text{far}}}$ are the hopping matrix elements, assumed to be negative. $a_l^\dagger$ and $a_l$ are the fermionic creation

Throughout this Supplementary document we refer to equations, sections, figures and table numbers of the main text using the **letter M prepended to the numbers**.

and annihilation operators, respectively. Each of the below specified eigenstates can be labelled by a unique dimensionless wave-number $\mathcal{K} \in [0, \pi]$. Other values of $\mathcal{K}$ would not yield a physically different eigenstate. The wave-number is related to the eigenenergy through the dispersion relation

$$\mathcal{E}(\mathcal{K}) = \epsilon + \sum_{n=1}^{N_{\text{far}}} 2t_n \cos(n\mathcal{K}). \tag{4}$$

Each of the eigenstates is conveniently expanded in the atomic-orbital basis set:

$$|\psi_{\mathcal{K}}\rangle = \sum_{l=1}^{\infty} \psi_{\mathcal{K},l} |l\rangle. \tag{5}$$

Each of the three sets derived below form a complete eigensystem of states satisfying the condition

$$\langle \psi_{\mathcal{K}} | \psi_{\mathcal{K}'} \rangle = \delta(\mathcal{K} - \mathcal{K}'). \tag{6}$$

## 1.1 $N_{\text{far}} = 1$

Eigenstates for this basic tight-binding model are well known and their components in the atomic-orbital basis take the form

$$\psi_{\mathcal{K},l} = \sqrt{\frac{2}{\pi}} \sin(\mathcal{K}l). \tag{7}$$

Physically they represent an equally weighted linear combination of an incoming and reflected wave. They form a non-degenerate set.

## 1.2 $N_{\text{far}} = 2$

Inclusion of 2nd NN interactions complicates the physics of the eigenstates and also their mathematical form. Dispersion relation (4) for this case can be written as

$$\mathcal{E}(\mathcal{K}) = \epsilon - 2t_2 + 2t_1 \cos\mathcal{K} + 4t_2 \cos^2\mathcal{K}. \tag{8}$$

The energy range $[\mathcal{E}_{\min}, \mathcal{E}_{\max}]$ available to the eigenstates is obtained by running $\mathcal{K}$ over the interval $[0, \pi]$. See also Sect. M2. Now we choose any single energy $\mathcal{E} \in [\mathcal{E}_{\min}, \mathcal{E}_{\max}]$ and find all possible inequivalent values of $\mathcal{K}$ that satisfy equation (8) for the given $\mathcal{E}$. This includes solving a quadratic equation for $\cos\mathcal{K}$. Apart from the real $\pm\mathcal{K}$ (and their periodic replicas) there are also complex wave-numbers found. They give rise to evanescent (or surface) states. We limit our discussion to cases without degeneracy (what is true for all relevant numerical values of $t_1$ and $t_2$). The complex wave-number

is then found to have a form

$$\hat{\mathcal{K}} = \pi + \mathrm{i}\kappa, \tag{9}$$

with $\kappa > 0$. Solutions with $-\kappa$ are mathematically correct but they do not satisfy the physical condition that the eigenstates have to be limited. Collecting the knowledge, the amplitudes of any of the physically correct eigenstates can be expressed by the formula

$$\psi_{\mathcal{K},l} = \sqrt{\frac{2}{\pi}} \left[\cos(\mathcal{K}l - \alpha) + (-1)^{l+1} e^{-\kappa l} \cos\alpha\right], \tag{10}$$

with

$$\alpha = \arctan\left(\frac{\cos\mathcal{K} + e^{\kappa}}{\sin\mathcal{K}}\right) \tag{11}$$

and

$$\kappa = \operatorname{arccosh}[-\cos(\mathcal{K}_-)], \tag{12}$$

$$\cos(\mathcal{K}_-) = -\frac{t_1}{4t_2} - \sqrt{\mathcal{D}}, \tag{13}$$

$$\mathcal{D} = \left(\frac{t_1}{4t_2}\right)^2 + \frac{\mathcal{E} - \epsilon}{4t_2} + \frac{1}{2}\ . \tag{14}$$

The ordinary wave-number $\mathcal{K} \equiv \mathcal{K}_+$ (with the sign coming from the associated branch when solving the quadratic equation) is for given $\mathcal{E}$ found from relation

$$\mathcal{K} = \arccos\left(-\frac{t_1}{4t_2} + \sqrt{\mathcal{D}}\right). \tag{15}$$

Eigenstates (10) form a non-degenerate set.

## 1.3 $N_{\text{far}} = 3$

We have also implemented the case with hoppings up to the 3rd NN included in the wires. Eigenstates of the semi-infinite wire for typically used values of parameters $t_1$, $t_2$, and $t_3$ now take the form

$$\psi_{\mathcal{K},l} = \sqrt{\frac{2}{\pi}} \left[\cos(\mathcal{K}l + \alpha) + B\cos(ql + \beta)e^{-\kappa l}\right] \tag{16}$$

and again are non-degenerate. We do not provide detailed description of the included parameters because the case of $N_{\text{far}} = 3$ is only marginally important for the present work; the effect of the 3rd NN in our study is negligible. Moreover, associated formulae for the parameters are rather lengthy and the components of the wave-numbers are found from solutions of a cubic equation. We mention that the amplitude $B$ is a positive real quantity.

## 2 Solution of the linear equations for the currents and electrostatic potentials

The linear regime assumed in Sect. M3.3.2 led to the set of the eight linear equations (M8), (M4), (M5), (M6a) and (M6b) for the seven unknown quantities $I_1, \ldots, I_4, U_2, U_3, U_4$. If the circuits conditions (M4) and (M5) are taken into account, the Eqs. (M8) for the 4-terminal device take the form

$$(G_{12}+G_{13}+G_{14})U_1 - G_{12}U_2 - G_{13}U_3 - G_{14}U_4 - I_1 = 0\,, \tag{17}$$

$$-G_{21}U_1 + (G_{21}+G_{23}+G_{24})U_2 - G_{23}U_3 - G_{24}U_4 + I_1 = 0\,, \tag{18}$$

$$-G_{31}U_1 - G_{32}U_2 + (G_{31}+G_{32}+G_{34})U_3 - G_{34}U_4 - I_3 = 0\,, \tag{19}$$

$$-G_{41}U_1 - G_{42}U_2 - G_{43}U_3 + (G_{41}+G_{42}+G_{43})U_4 + I_3 = 0\,. \tag{20}$$

After inclusion of the TRS [Eq. (M2)] these four equations are found linearly dependent in a simple manner: adding together first two of them would provide us with the same equation as adding together the second two of them. The resulting equation, to be used later on, is

$$(G_{31}+G_{41})U_1 + (G_{32}+G_{42})U_2 - (G_{13}+G_{23})U_3 - (G_{14}+G_{24})U_4 = 0\,. \tag{21}$$

We still have available the ground-level condition (M7) (see Fig. M2), which we apply now without any relevant loss of generality. We will restore $U_1$ in our final results. From the Eq. (21) we express

$$U_3 = \frac{G_{32}+G_{42}}{G_{13}+G_{23}}\,U_2 - \frac{G_{14}+G_{24}}{G_{13}+G_{23}}\,U_4 \equiv c_2U_2 - c_4U_4\,. \tag{22}$$

On the right-hand side of the Eq. (22) we have introduced the constants

$$c_2 \equiv \frac{G_{32}+G_{42}}{G_{13}+G_{23}}\,, \qquad c_4 \equiv \frac{G_{14}+G_{24}}{G_{13}+G_{23}}\,. \tag{23}$$

We first express currents $I_1$ and $I_3$ as some (linear) functions of the two potentials: substitution of the expression (22) for $U_3$ into the Eqs. (17) and (20) (with $U_1 = 0$) gives us a pair of linear equations

$$\left(G_{12} + \frac{G_{32}+G_{42}}{G_{13}+G_{23}}\,G_{13}\right)U_2 + \left(G_{14} - \frac{G_{14}+G_{24}}{G_{13}+G_{23}}\,G_{13}\right)U_4 = -I_1\,, \tag{24a}$$

$$\left(G_{42} + \frac{G_{32}+G_{42}}{G_{13}+G_{23}}\,G_{43}\right)U_2 - \left(G_{41}+G_{42}+G_{43} + \frac{G_{14}+G_{24}}{G_{13}+G_{23}}\,G_{43}\right)U_4 = I_3\,, \tag{24b}$$

i.e. we now have available explicit formulae

$$I_1 = I_1(U_2, U_4)\,, \qquad I_3 = I_3(U_2, U_4)\,. \tag{25}$$

From this point we switch the notation for currents and to use $I_{\mathrm{A}}$ instead of $-I_1 = I_2$ and $I_{\mathrm{B}}$ instead of $-I_3 = I_4$:

$$I_{\mathrm{A}} \equiv I_2\,, \qquad I_{\mathrm{B}} \equiv I_4\,. \tag{26}$$

The externally controllable mutually independent variables are the two bias voltages $V_{\mathrm{A}}$ and $V_{\mathrm{B}}$, not the potentials $U_2$, $U_4$. There are also the two resistors in the circuits. Our aim is to find the electric currents $I_{\mathrm{A}}$ and $I_{\mathrm{B}}$ flowing through the leads at the terminals 2 and 4 as functions of the bias voltages $V_{\mathrm{A}}$ and $V_{\mathrm{B}}$. To accomplish the goal we relate the potentials $U_2$ and $U_4$ to the bias voltages $V_{\mathrm{A}}$ and $V_{\mathrm{B}}$ using Kirchhoff's second law (M6). Relation (M6b) for $U_4$ includes potential $U_3$, which is another unknown variable and has to be expressed as $U_3 = U_3(U_2, U_4)$ using the Eq. (22). Accomplishing this calculation we obtain an expression for $U_4$ which we put down together with the Eq. (M6a) for $U_2$, now simplified due to the choice (M7).

$$U_2 = V_{\mathrm{A}} - R_{\mathrm{A}} I_{\mathrm{A}}\,, \tag{27a}$$

$$U_4 = \frac{1}{1+c_4}\left(c_2 V_{\mathrm{A}} - c_2 R_{\mathrm{A}} I_{\mathrm{A}} + V_{\mathrm{B}} - R_{\mathrm{B}} I_{\mathrm{B}}\right). \tag{27b}$$

These forms will be inserted into the linear set (24). To do this, we introduce another abbreviated notation: the linear set (24) will be written as

$$a U_2 + b U_4 = I_{\mathrm{A}}\,, \tag{28a}$$

$$c U_2 - d U_4 = -I_{\mathrm{B}}\,, \tag{28b}$$

where

$$a \equiv G_{12} + \frac{G_{32}+G_{42}}{G_{13}+G_{23}}\, G_{13} \equiv\; G_{12} + c_2 G_{13}\,, \tag{29a}$$

$$b \equiv G_{14} - \frac{G_{14}+G_{24}}{G_{13}+G_{23}}\, G_{13} \equiv\; G_{14} - c_4 G_{13}\,, \tag{29b}$$

$$c \equiv G_{42} + \frac{G_{32}+G_{42}}{G_{13}+G_{23}}\, G_{43} \equiv\; G_{42} + c_2 G_{43}\,, \tag{29c}$$

$$d \equiv \qquad\qquad\qquad \equiv\; G_{41} + G_{42} + (1+c_4) G_{43}\,. \tag{29d}$$

Now we accomplish the substitution of (27) into the abbreviated linear set (28):

$$a(V_{\rm A} - R_{\rm A} I_{\rm A}) + b\left[\frac{1}{1+c_4}(c_2 V_{\rm A} - c_2 R_{\rm A} I_{\rm A} + V_{\rm B} - R_{\rm B} I_{\rm B})\right] = I_{\rm A}\,, \tag{30a}$$

$$c(V_{\rm A} - R_{\rm A} I_{\rm A}) - d\left[\frac{1}{1+c_4}(c_2 V_{\rm A} - c_2 R_{\rm A} I_{\rm A} + V_{\rm B} - R_{\rm B} I_{\rm B})\right] = -I_{\rm B}\,. \tag{30b}$$

After regrouping of the terms and denoting

$$\frac{1}{1+c_4} \equiv c_4' \tag{31}$$

we obtain

$$[1 + (a + bc_4' c_2) R_{\rm A}] I_{\rm A} + \qquad bc_4' R_{\rm B} I_{\rm B} = \quad (a + bc_4' c_2) V_{\rm A} + bc_4' V_{\rm B}\,, \tag{32a}$$

$$(-c + dc_4' c_2) R_{\rm A} I_{\rm A} + (1 + dc_4' R_{\rm B}) I_{\rm B} = (-c + dc_4' c_2) V_{\rm A} + dc_4' V_{\rm B}\,. \tag{32b}$$

Solving this pair of the linear equations for the unknown currents $I_{\rm A}$ and $I_{\rm B}$ we get linear relations

$$I_{\rm A} = I_{\rm A}(V_{\rm A}, V_{\rm B})\,, \qquad I_{\rm B} = I_{\rm A}(V_{\rm A}, V_{\rm B})\,. \tag{33}$$

After performing series of algebraic manipulations with multiple use of the TRS relations

$$\sum_{\beta(\neq\alpha)} G_{\alpha\beta} = \sum_{\beta(\neq\alpha)} G_{\beta\alpha} \tag{34}$$

we finally obtain the explicit formulae (M9). The determinant of the left hand side of the linear system (32) is actually the expression $D(G,R)$ given by the Eq. (M12). Büttiker's conductances entering our formulae for the system with the resistances are given by expressions [1]

$$\alpha_{\rm AA} = \frac{1}{S}\left[S_1 S - (G_{13} + G_{14})(G_{31} + G_{41})\right], \tag{35a}$$

$$\alpha_{\rm AB} = \frac{1}{S}(G_{13} G_{24} - G_{14} G_{23})\,, \tag{35b}$$

$$\alpha_{\rm BA} = \frac{1}{S}(G_{31} G_{42} - G_{41} G_{32})\,, \tag{35c}$$

$$\alpha_{\rm BB} = \frac{1}{S}\left[S_3 S - (G_{31} + G_{32})(G_{13} + G_{23})\right], \tag{35d}$$

with

$$S \;=\; G_{13} + G_{23} + G_{14} + G_{24} \;=\; G_{31} + G_{32} + G_{41} + G_{42} \tag{36}$$

and

$$S_\alpha = \sum_{\beta\neq\alpha} G_{\alpha\beta} = \sum_{\beta\neq\alpha} G_{\beta\alpha} = \frac{2e^2}{h}\left(N_\alpha - \mathcal{T}_{\alpha\leftarrow\alpha}\right). \tag{37}$$

$N_\alpha$ is the number of channels per electrode $\alpha$. In our model it is the number of the elementary wires composing the electrode $\alpha$. We find that Büttiker's conductances $\alpha_{CC'}$ can alternatively be expressed by formulae

$$\alpha_{\mathrm{AA}} = S_1 \;\; - \frac{1}{S}\,(S_1 - G_{12})(S_1 - G_{21}), \tag{38a}$$

$$\alpha_{\mathrm{AB}} = G_{13} - \frac{1}{S}\,(S_1 - G_{12})(S_3 - G_{43}), \tag{38b}$$

$$\alpha_{\mathrm{BA}} = G_{31} - \frac{1}{S}\,(S_1 - G_{21})(S_3 - G_{34}), \tag{38c}$$

$$\alpha_{\mathrm{BB}} = S_3 \;\; - \frac{1}{S}\,(S_3 - G_{34})(S_3 - G_{43}) \tag{38d}$$

and satisfy relation

$$(\alpha_{\mathrm{AA}} - S_1)(\alpha_{\mathrm{BB}} - S_3) = (\alpha_{\mathrm{AB}} - G_{13})(\alpha_{\mathrm{BA}} - G_{31}). \tag{39}$$

Formulae for the electrostatic potentials differences, for instance the Eq. (M11), are found as follows. Using the Eqs. (M6), (M7) and (M9) we first find the potentials differences (see also Fig. M2)

$$U_2 - U_1 = \frac{(1 + \alpha_{\mathrm{BB}} R_{\mathrm{B}}) V_{\mathrm{A}} + \alpha_{\mathrm{AB}} R_{\mathrm{A}} V_{\mathrm{B}}}{1 + \alpha_{\mathrm{AA}} R_{\mathrm{A}} + \alpha_{\mathrm{BB}} R_{\mathrm{B}} + \gamma R_{\mathrm{A}} R_{\mathrm{B}}}, \tag{40a}$$

$$U_4 - U_3 = \frac{(1 + \alpha_{\mathrm{AA}} R_{\mathrm{A}}) V_{\mathrm{B}} + \alpha_{\mathrm{BA}} R_{\mathrm{B}} V_{\mathrm{A}}}{1 + \alpha_{\mathrm{AA}} R_{\mathrm{A}} + \alpha_{\mathrm{BB}} R_{\mathrm{B}} + \gamma R_{\mathrm{A}} R_{\mathrm{B}}}, \tag{40b}$$

restoring in this way the reference potential $U_1$, which can be set to an arbitrary value and the explicit presence of which allows us to write more general and symmetrical formulae. Next we determine the potentials differences in the perpendicular direction and across the sample. To achieve this goal, we first use the Eq. (28a), which yields $U_4 = (I_{\mathrm{A}} - aU_2)/b$ for $U_1 = 0$. $U_2$ is already know from the Eq. (40a). Accomplishing lengthy algebraic manipulations with multiple use of the TRS relations of the form (M2)

and finally restoring the reference potential $U_1$ we arrive at

$$\begin{aligned} U_4 - U_2 = -\frac{1}{SD(G,R)} \big[ & (G_{31}+G_{41})V_{\mathrm{A}} + (G_{41}S_3 + G_{31}G_{43})R_{\mathrm{B}}V_{\mathrm{A}} \\ & -(G_{13}+G_{23})V_{\mathrm{B}} - (G_{23}S_1 + G_{13}G_{21})R_{\mathrm{A}}V_{\mathrm{B}} \big], \end{aligned} \tag{41a}$$

$$\begin{aligned} U_3 - U_1 = \frac{1}{SD(G,R)} \big[ & (G_{42}+G_{32})V_{\mathrm{A}} + (G_{32}S_4 + G_{42}G_{34})R_{\mathrm{B}}V_{\mathrm{A}} \\ & -(G_{24}+G_{14})V_{\mathrm{B}} - (G_{14}S_2 + G_{24}G_{12})R_{\mathrm{A}}V_{\mathrm{B}} \big] \end{aligned} \tag{41b}$$

(the differences in the perpendicular direction) and

$$\begin{aligned} U_4 - U_1 = \frac{1}{SD(G,R)} \big[ & (G_{32}+G_{42})V_{\mathrm{A}} + (G_{42}S_3 + G_{32}G_{43})R_{\mathrm{B}}V_{\mathrm{A}} \\ & +(G_{23}+G_{13})V_{\mathrm{B}} + (G_{13}S_2 + G_{23}G_{12})R_{\mathrm{A}}V_{\mathrm{B}} \big], \end{aligned} \tag{42a}$$

$$\begin{aligned} U_3 - U_2 = -\frac{1}{SD(G,R)} \big[ & (G_{41}+G_{31})V_{\mathrm{A}} + (G_{31}S_4 + G_{41}G_{34})R_{\mathrm{B}}V_{\mathrm{A}} \\ & +(G_{14}+G_{24})V_{\mathrm{B}} + (G_{24}S_1 + G_{14}G_{21})R_{\mathrm{A}}V_{\mathrm{B}} \big] \end{aligned} \tag{42b}$$

(the potentials differences across the sample). Only one of the four Eqs. (41) and (42) is needed to be derived by the algebraic manipulations. The other three follow from the symmetry of the scheme (Fig. M2) upon performing exchanges of the respective indices and of the bias voltages signs.

# 3 Solution of the non-linear equations for the currents and electrochemical potentials

In Sects. M2 and M3.3.1 the scheme according to Fig. M2 has been defined. The solution to the corresponding equations in the linear regime was found in Sect. M3.3.2 and in Sect. 2. In Sect. M3.3.3 we described how the task is solved in the non-linear regime where the dependence of the transmission matrix on the energy has to be taken into account. Here we provide additional details to this procedure. Like in the linear regime [c.f. the Eqs. (32)] we now obtain equations

$$[1 + (a + bc_4'c_2)R_{\mathrm{A}}]\,\delta I_{\mathrm{A}} + bc_4'R_{\mathrm{B}}\,\delta I_{\mathrm{B}} = (a + bc_4'c_2)\,\delta V_{\mathrm{A}} + bc_4'\,\delta V_{\mathrm{B}}\,, \tag{43a}$$

$$(-c + dc_4'c_2)R_{\mathrm{A}}\,\delta I_{\mathrm{A}} + (1 + dc_4'R_{\mathrm{B}})\,\delta I_{\mathrm{B}} = (-c + dc_4'c_2)\,\delta V_{\mathrm{A}} + dc_4'\,\delta V_{\mathrm{B}}\,, \tag{43b}$$

which have their structure identical to the Eqs. (32). Individual coefficients in the Eqs. (43) now include the conductance matrix elements at three different energies indi-

cated by the superscript:

$$c_2 \equiv \frac{G_{32}^{(2)} + G_{42}^{(2)}}{G_{13}^{(3)} + G_{23}^{(3)}}\,, \qquad c_4 \equiv \frac{G_{14}^{(4)} + G_{24}^{(4)}}{G_{13}^{(3)} + G_{23}^{(3)}}\,. \tag{44}$$

$$a \equiv G_{12}^{(2)} + \frac{G_{32}^{(2)} + G_{42}^{(2)}}{G_{13}^{(3)} + G_{23}^{(3)}} G_{13}^{(3)} \equiv G_{12}^{(2)} + c_2 G_{13}^{(3)}\,, \tag{45a}$$

$$b \equiv G_{14}^{(4)} - \frac{G_{14}^{(4)} + G_{24}^{(4)}}{G_{13}^{(3)} + G_{23}^{(3)}} G_{13}^{(3)} \equiv G_{14}^{(4)} - c_4 G_{13}^{(3)}\,, \tag{45b}$$

$$c \equiv G_{42}^{(2)} + \frac{G_{32}^{(2)} + G_{42}^{(2)}}{G_{13}^{(3)} + G_{23}^{(3)}} G_{43}^{(3)} \equiv G_{42}^{(2)} + c_2 G_{43}^{(3)}\,, \tag{45c}$$

$$d \equiv \qquad \equiv G_{41}^{(4)} + G_{42}^{(4)} + (1 + c_4) G_{43}^{(3)}\,. \tag{45d}$$

$c_4'$ used in the Eqs. (43) is again defined by the expression (31) but now with the more general $c_4$ according to the Eq. (44). The precise meaning of the superscript notation is defined by

$$G_{\alpha\beta}^{(\gamma)} \equiv \frac{2e^2}{h}\, \mathcal{T}_{\alpha\leftarrow\beta}(\mu_\gamma)\,, \tag{46}$$

i.e. the upper index of $G_{\alpha\beta}$ marks the value of the electrochemical potential at which the conductance has to be evaluated.

If we now, for a fixed set of known functions $G_{\alpha\beta}(u)$, aim to calculate the currents $I_{\mathrm{A}}$ and $I_{\mathrm{B}}$ at given bias voltages $V_{\mathrm{A}}$ and $V_{\mathrm{B}}$, we start from zero voltages and in small steps $\delta V_{\mathrm{A}}$ and $\delta V_{\mathrm{B}}$ increase them up to their final values $V_{\mathrm{A}}$ and $V_{\mathrm{B}}$. The path in the $(V_{\mathrm{A}}, V_{\mathrm{B}})$ space can be arbitrary. The procedure is numerically stable for all examined cases and requires almost negligible computational time in comparison to that used to compute the spectra of $G_{\alpha\beta}(u)$.

# 4 Nanoribbons with the cut-outs vs. the intact nanoribbon

## 4.1 Linear-response conductance matrices at the neutrality point

In main text we consider the four-terminal nanojunction with the explicit circuits. As particular examples we use the junctions based either on the intact graphene nanoribbon (GNR) or on the GNR with the 60-atom cut-out [Figs. M1 and M3(b)]. Concerning the linear-response regime, we demonstrated the transport properties of the setups both at

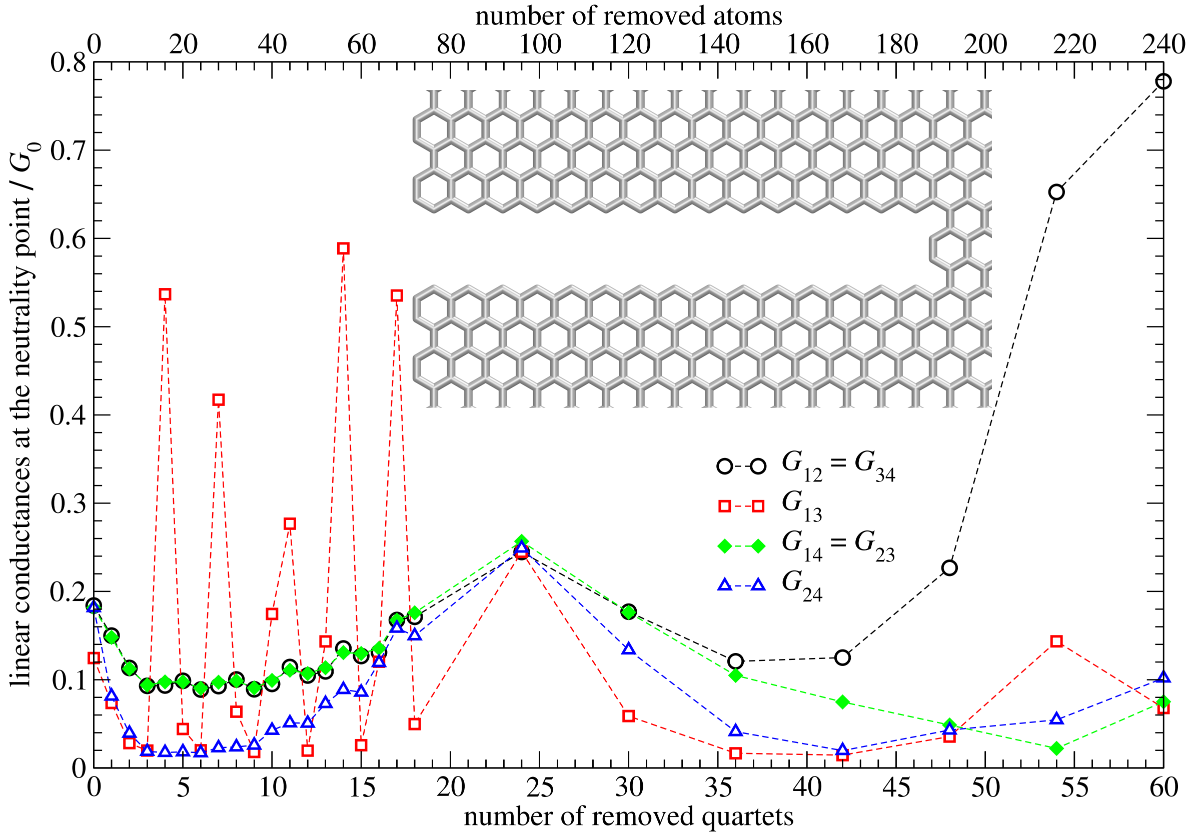


Figure 1: The linear conductances computed at the *neutrality point* (no gate voltage) for a set of 26 graphene structures based on the GNR shown in Fig. M1. The individual structures differ by the depth of the cut-out, which is quantified by the number of the removed atoms (the upper x axis). In each of the structures this number is an integral multiply of 4 hence it is convenient to quantify the depth of the cut-out by the number of removed quartets. The particular example shown in the inset is a detail of the structure having the 60-atom (15 quartets) cut-out. This perturbed structure was considered also in main text together with the intact GNR (a special case having the zero cut-out); data for these two structures are also shown in the graph. Below we provide more detailed results also to the structures with 14 and 16 removed quartets including the case of the resonantly increased conductance due to the ZZ edge states when a gate voltage is applied.

the neutrality point as well as in the regime with the applied gate voltage. The gate voltage allowed us to study the regime of resonantly increased conductance along the zig-zag (ZZ) edges.

Different perturbations to the original intact GNR lead to different conductance properties of such a junction. A removal of even one atom may modify the conductance matrix substantially. Although exploration of various perturbations and defects and their impact were not the purpose of our paper, we at least provide a representative set of results for the kind of the perturbation (the cut-out) introduced in main text. In Fig. 1 we provide our results for the 4-point linear conductance at the *neutrality point* only (no gate voltage) for 26 graphene structures with the cut-out of the shape

as shown in the inset. The caption to the figure provides a more detailed description. Not surprisingly, the matrix element most affected by the increasing cut-out is $G_{13}$ (the red squares in the graph; Fig. M1 defines the numbering of the corners). The matrix element sharply oscillates as a function of the number of removed quartets. The periodicity with which the high (or low) values of $G_{13}$ occur, is 3 quartets; for example, a low value occurs at the numbers 12, 15 and 18 removed quartets, among the other numbers. For the numbers above 18 we only have calculated the cases when the number of the removed quartets corresponds to a low $G_{13}$ magnitude (at least in comparison to $G_{12}$). We note that the periodicity of 3 occurs also in the case of perfect armchair graphene nanoribbons (AGNRs). It is well known that they can be classified into three different classes: (i) highly conductive (small gap, metallic), (ii) semiconducting (medium gap) and (iii) insulating (largest gap)[1], depending on the width of an AGNR [2, 3]. The structures with the cut-out considered in our work have more complicated shapes than just AGNRs and in addition we consider the four-point conductance. Still, the periodicity of 3 is the same as found in Refs. [2, 3]. As for the size of the GNR considered in the present work, its dimensions are $(143, 42)$ according to the convention used in Ref. [4]. $143 = 3p - 1$ with and integral $p$ which means that the ribbon considered in our paper belongs to the metallic class if considered as an AGNR. The total GNR length corresponds to 71 quartets plus two additional atoms.

### 4.2 I/V plots: the neutrality point vs. the gate field induced resonant regime or coupled vs. independent circuits

In main text we presented Fig. M3, which in terms of the currents described the transport properties of the intact and the perturbed GNR with particular emphasise on the mutual interaction between the two classical circuits through the quantum subsystem (the GNR). The same kind of comparisons in the linear regime was demonstrated in Fig. M7 for the case of the resonantly increased conductance along the ZZ edges due to the applied gate voltage. As said above, the perturbed structure considered in main text had the 15-quartets cut-out. To provide a more complete picture, we accomplished the same kind of the circuit analysis for two additional perturbed GNRs: the one with the 14 quartets removed (a high $G_{13}$) and the GNR with the 16-quartet cut-out (a medium $G_{13}$); see Fig. 1. For convenience we also include the cases of the perfect GNR and the one with the 15 removed quartets, which were also shown in main text. The results are displayed in the panes of Fig. 2. Its panes (a) and (c) show the same data as Fig. M3, although now using a larger vertical axis range. Similarly, the panes (e) and (g) show the same data as Fig. M7. A distinct feature, not characteristic for the result in main text, is the negative slope of the $I_{\mathrm{A}}$ vs. $V_{\mathrm{B}}$ plots in Fig. 2(b). The negative differential

[1] The gaps however decrease with the GNR's size along the armchair direction.

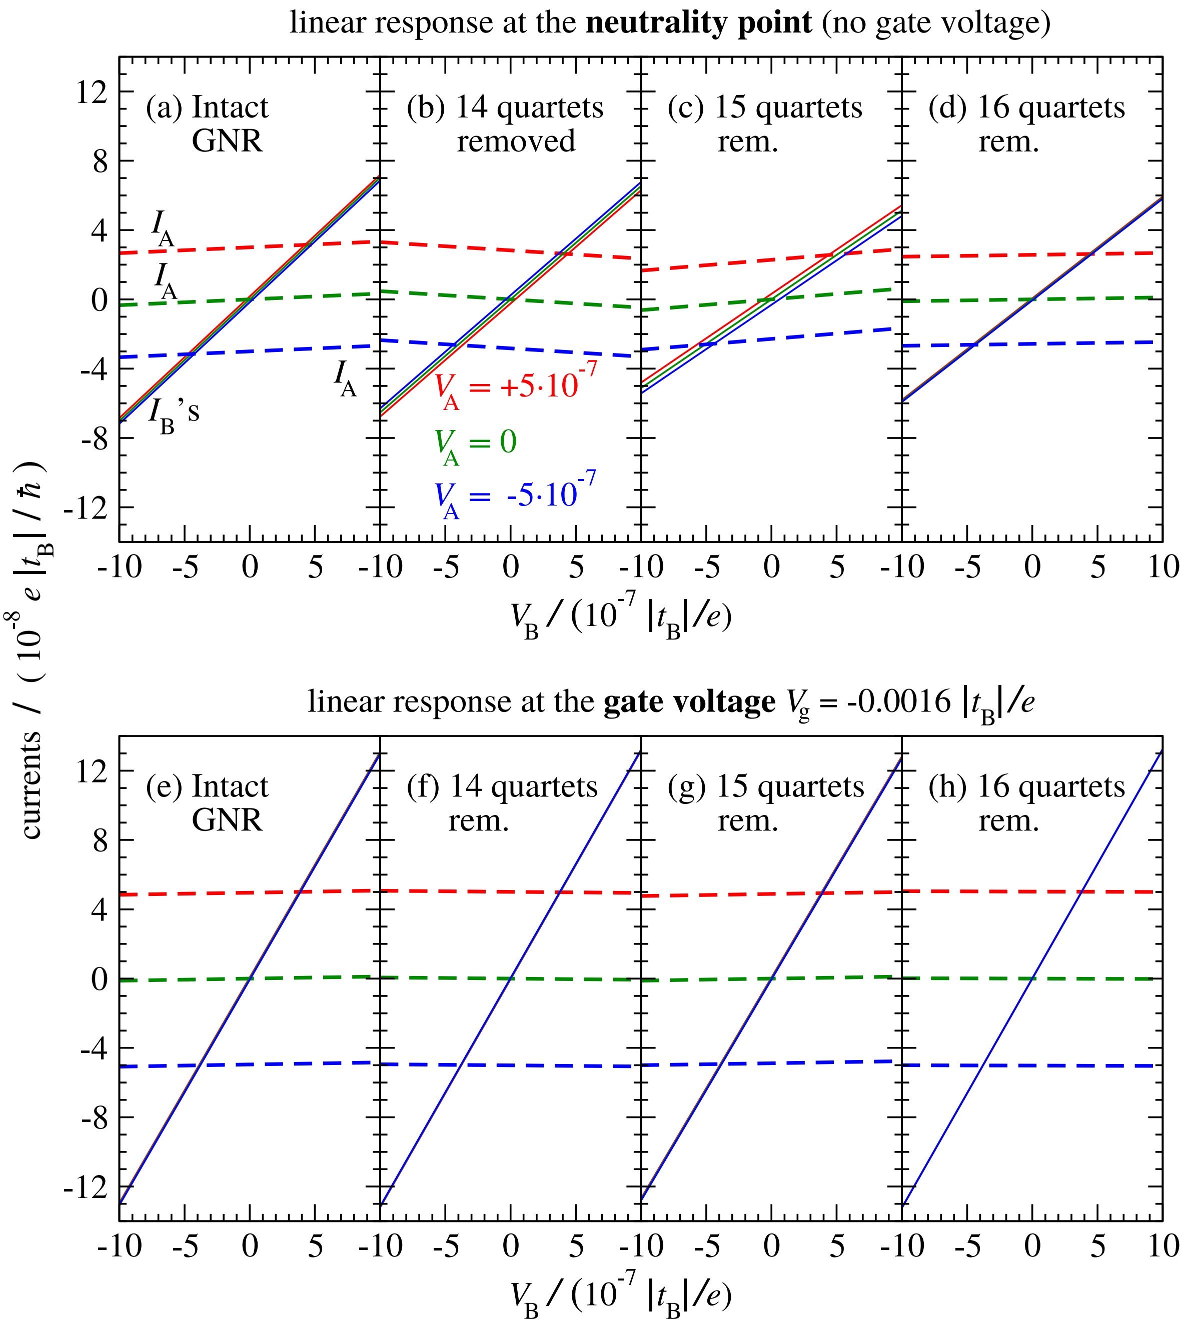


Figure 2: Same kind of plots as in Figs. M1 and M7 but now including two additional perturbed GNRs, (the cases of 14 and 16 removed quartets) and using a common scale for the vertical axes. The legends $I_A$, $I_B$'s and $V_A$ apply to all 8 panes. Each pane contains three $I_A$ plots and three $I_B$ plots although the latter ones may be indistinguishable, especially on graphs (e)-(h), which represent the cases of the resonantly increased conductance due to the ZZ edge modes. The units of the bias voltage $V_A$ are $|t_B|/e$. All conditions like the assumed resistances $R_A$ and $R_B$ are the same as in main text. The eight panes of this figure are based on the eight sets of data shown in Tab. 1.

conductance is caused by the large matrix element $G_{13}$ for this case; cf. Fig. 1 and also Tab. 1, which is a superset of Tab. M1. Another interesting feature is that in the resonant regime the conductances along the ZZ edges ($G_{12} = G_{34}$) are so large that

Table 1: A superset to Tab. M1. The extended table here includes the matrix elements for the two additional structures – the perturbed GNRs characterised by the 14 and 16 removed quartets (56 and 64 removed atoms). These eight sets of data correspond to the eight panes of Fig. 2.

| | $G_{12}$ | $G_{13}$ | $G_{14}$ | $G_{24}$ |
|---|---|---|---|---|
| Intact | 0.1840 | 0.1246 | 0.1816 | 0.1246 |
| Pert.14 | 0.1354 | 0.5887 | 0.1307 | 0.08884 |
| Pert.15 | 0.1269 | 0.02575 | 0.1297 | 0.08584 |
| Pert.16 | 0.1310 | 0.1204 | 0.1355 | 0.1195 |
| Intact $+V_g$ | 1.012 | 0.07974 | 0.1567 | 0.07974 |
| Pert.14$+V_g$ | 0.9372 | 0.3526 | 0.2109 | 0.1828 |
| Pert.15$+V_g$ | 0.9180 | 0.07857 | 0.1859 | 0.1679 |
| Pert.16$+V_g$ | 0.9658 | 0.2500 | 0.2097 | 0.2011 |

the nanoribbon edges operate as almost two independent conductors, irrespectively of a particular perturbation of the armchair edge.

# 5 Linear vs. non-linear regime (with the equilibrium-based transmission spectra)

In this supplementary section we assume the following conditions:

- the perfect (intact) GNR (Fig. M1)
- zero gate field
- relatively high bias voltages so that the non-linear regime is reached
- We account for the energy-dependence of the conductance matrix, which is shown in Fig. M5(a).
- We use just this single (fixed) set of the conductance matrix spectra, obtained using the full equilibrium conditions. Hence the effect of non-equilibrium Fermi levels in the leads is not included in this section, in particular in its Fig. 3.

The dependence of the current $I_{\text{max}}$ (defined below) on the resistance (with the fixed ratio $R_A/R_B = 7.3/4.9$) is semi-quantitatively displayed in Fig. 3 using the black line with circles. Here the value of $R$ used for the descriptions of the horizontal axis is the arithmetic average between $R_A$ and $R_B$. $I_{\text{max}}$ on the vertical axis is the maximum chosen among the currents $I_A$ and $I_B$ for given $R_A$ and $R_B$ on the examined domain of the bias voltages: $V_A \in \{0,\ 2\cdot 10^{-3}\,|t_B|/e\}$, $V_B \in [0,\ 2\cdot 10^{-3}\,|t_B|/e]$. The value of $G^{\text{edge}}$ typed within the graph serves only for comparison purposes, i.e. what is the actual resistance $R$ in comparison to the typical inverse conductance of the ZZ edge.

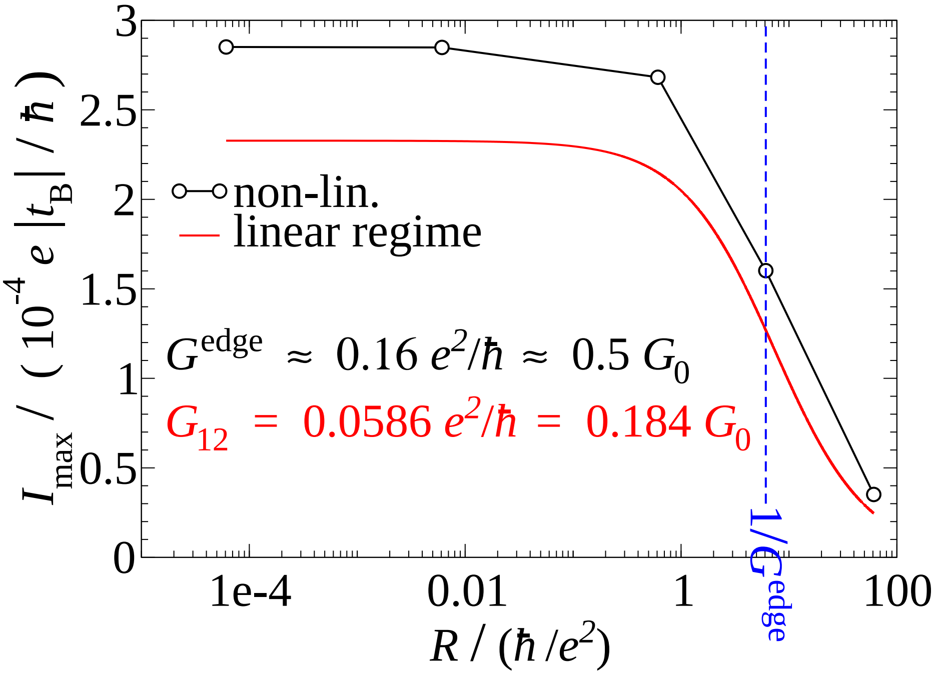


Figure 3: Results for the intact GNR (Fig. M1) with no gate voltage. Black line with circles: maximum of any of the currents $I_{\rm A}$ and $I_{\rm B}$ versus resistance. The maxima are determined on the chosen domain of the bias voltages, $V_{\rm A} \in \{0,\ 2\cdot 10^{-3}\,|t_{\rm B}|/e\}$, $V_{\rm B} \in [0,\ 2\cdot 10^{-3}\,|t_{\rm B}|/e]$. The resistance $R$ is the arithmetic average of the $R_{\rm A}$ and $R_{\rm B}$ resistances, which are always chosen in the same ratio $R_{\rm A}/R_{\rm B} = 7.3/4.9$. $G^{\rm edge}$ is a typical $G_{12}$ or $G_{34}$ conductance value along the ZZ edges such as can be seen also in Fig. M5. The vertical dashed line marks the value of $1/G^{\rm edge}$ on the resistance axis. For comparison, analytical results for the linear regime are outlined with the smooth red line. They result from the formulae (M9) and employ the conductance matrix from the first row of Tab. M1 (also Tab. 1). In the context of the nomenclature of Sect. 6 here (also of Sects. M3.3.4 and M4.2), the black line with circles was obtained at the ITER1 level of approximation.

For another comparison, in the same graph we in addition provide the plot for the linear regime (the smooth red line). It results from the formulae (M9), with the conductance matrix from the fist row of Tab. M1 (also Tab. 1) and assuming $V_{\rm A} = V_{\rm B} = 2{\cdot}10^{-3}\,|t_{\rm B}|/e$. These bias voltages are too high for the linear regime but still the results calculated in this way (solid red line in Fig. 3) present a convenient analytically obtained reference to the numerical results for the non-linear regime (the black plot with circles).

# 6 The composite system beyond equilibrium: iterations toward self-consistency

In Sect. M4.2 the results in terms of the currents are shown up to the ITER4 level of our recursive scheme (Fig. M6). In Fig. 4 we provide direct comparison of the *currents* computed at different levels of the approximation. All assumptions here are identical to

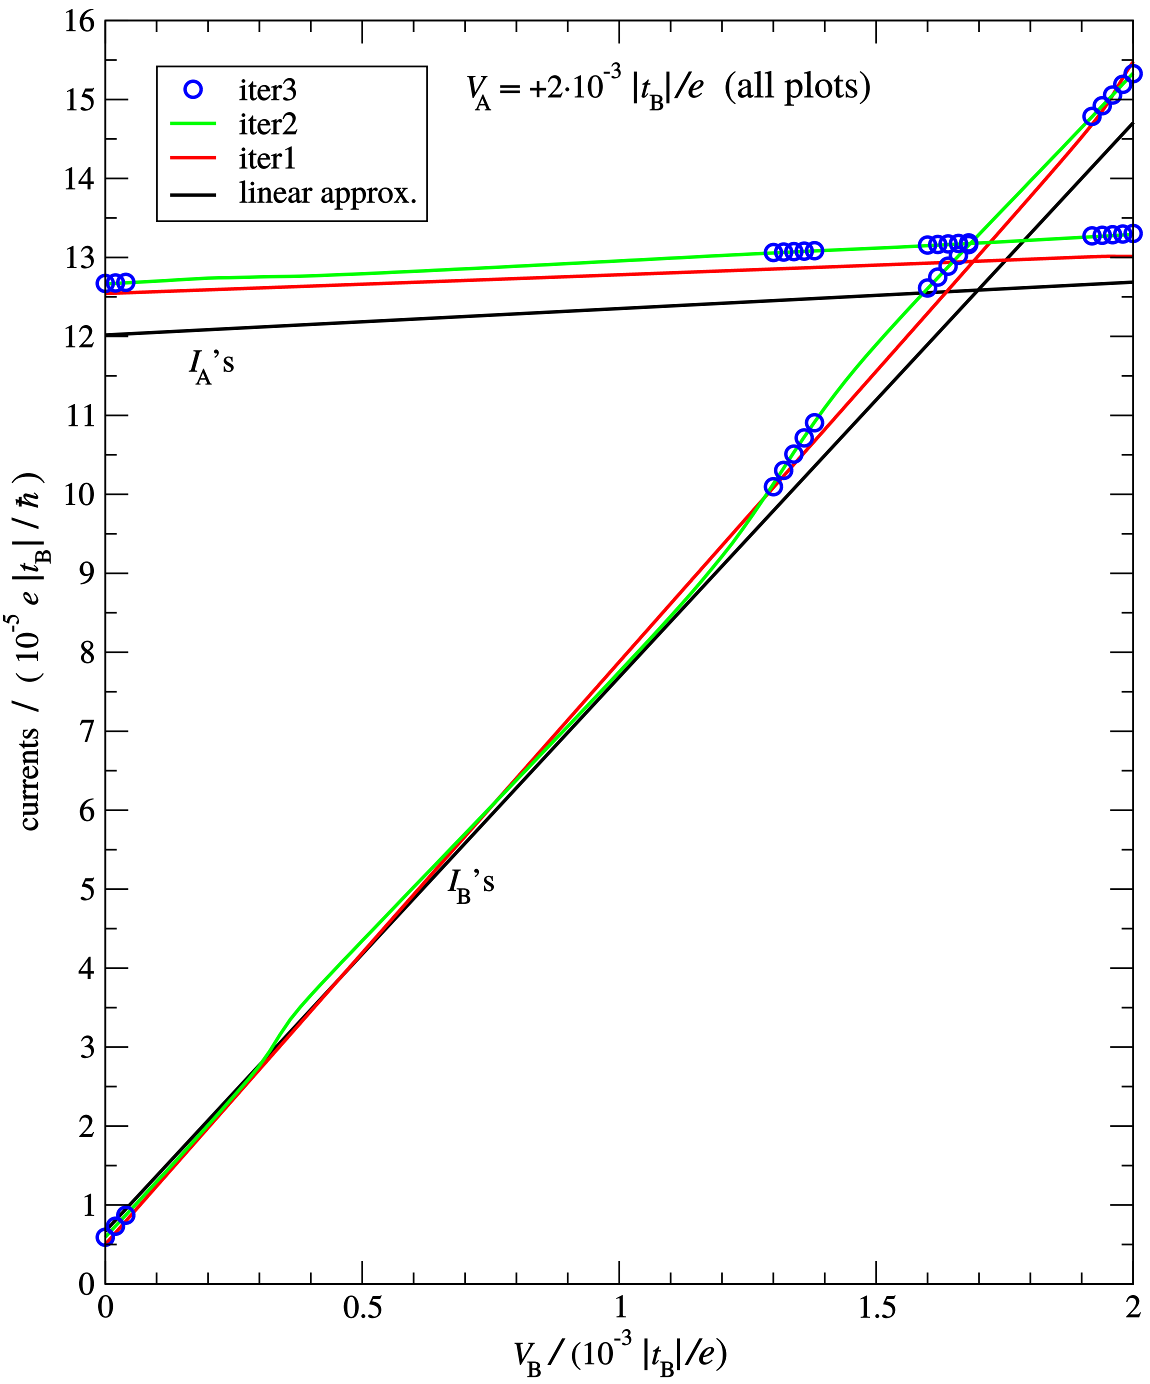


Figure 4: Comparison of the subsequent iterations towards the self-consistency of the currents and the electrochemical potentials. These plots extend Fig. M6(b). The bias voltage in circuit A is assumed to be fixed at the shown value. More description can be found in Sect. 6. The electrochemical potentials vs. the $V_{\rm B}$ voltage are shown in Fig. 5 below.

those assumed in Sect. M4.2 (including Fig. M6), namely the perfect GNR, zero gate field and the values of the resistances.

The black I/V plots in Fig. 4 are straight lines obtained using the linear-response approximation, namely the Eqs. (M9), with the conductance matrix, which was also used for Figs. M3(a) and M4 and also for Fig. 2(a). (The matrix elements are listed

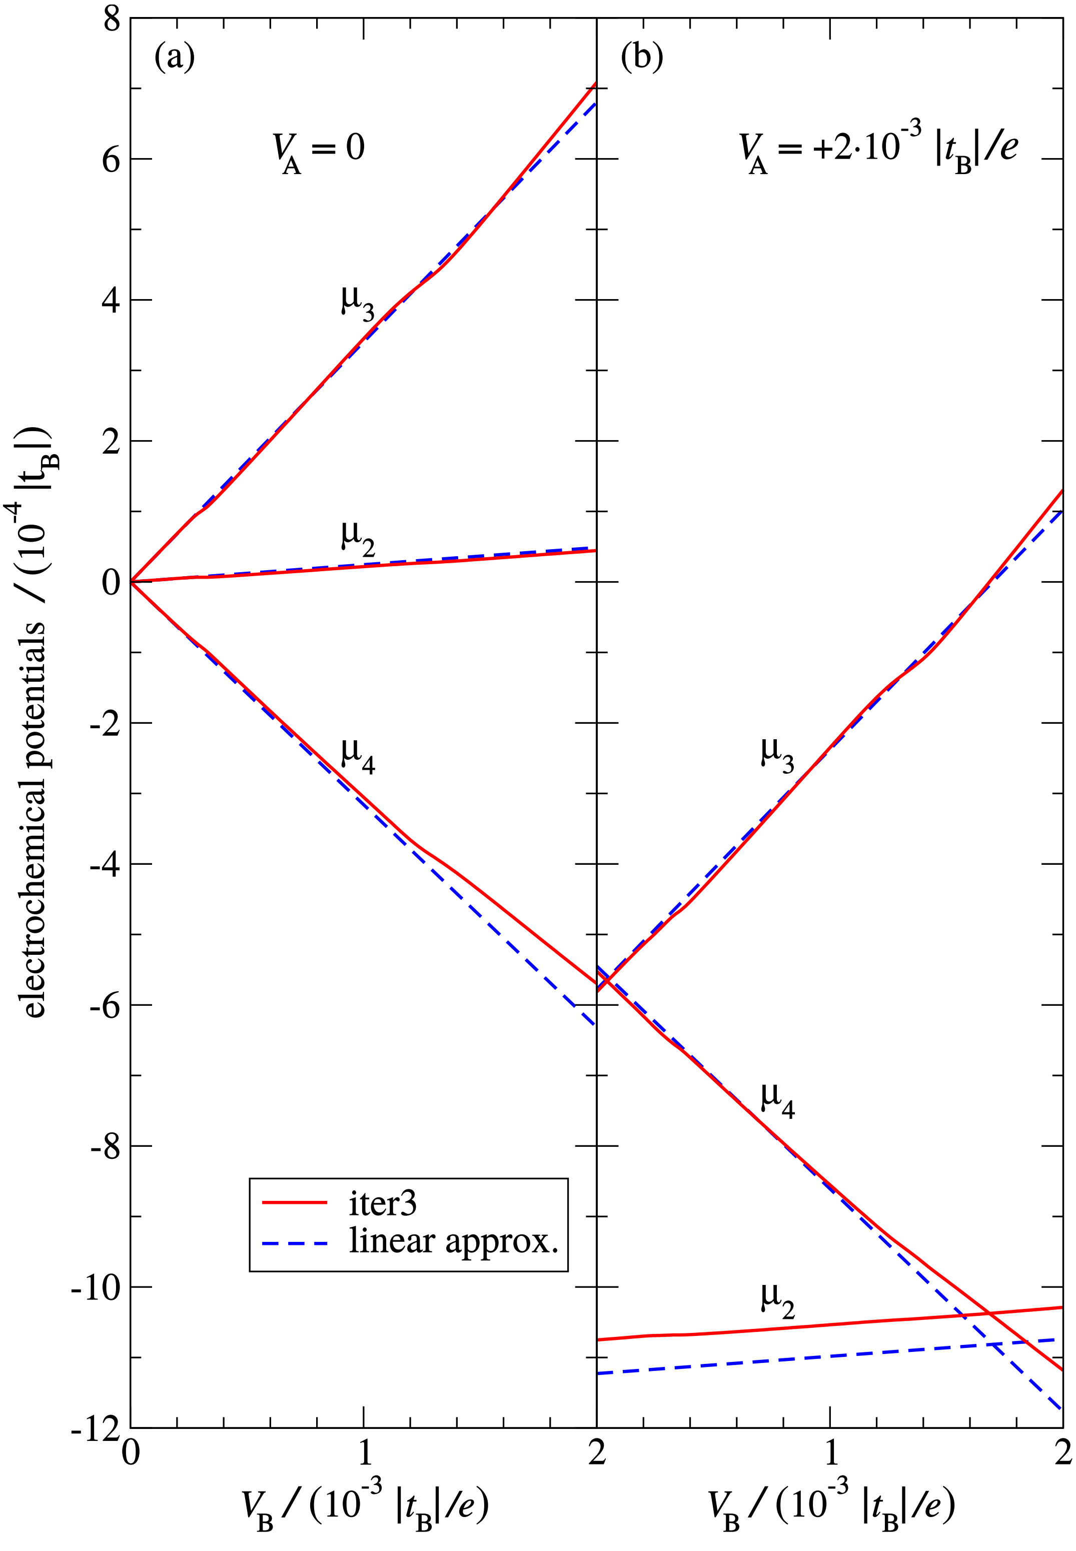


Figure 5: The electrochemical potentials of the leads vs. the bias voltage in circuit B, computed for the intact GNR at the same conditions as were assumed for Fig. M6. (a) The case of zero bias voltage in circuit A. (b) The case of the elevated bias voltage $V_A$. Results at two levels of the approximation are shown: the linear-response model (the straight lines, dashed) and the potentials at the ITER3 level. $\mu_\alpha = -eU_\alpha$ is the electrochemical potential in lead $\alpha$, $U_\alpha$ being the corresponding electrostatic potential. $\mu_1 \equiv 0$ by definition of the scheme's ground level (Fig. M2). See also Fig. M6(a) and Fig. M6(d) where the corresponding currents at the ITER3 level are outlined. Complementary results on the currents can be found also in Fig. 4.

in the first row of Tab. M1 as well as in Tab. 1.) Although the linear approximation becomes worse for higher voltages, we still present it in the graph as an appropriate reference (the black lines in Fig. 4).

The ITER1 curves in Fig. 4 (the red lines) already assume the non-linear regime, although using the fixed set of the conductance matrix spectra. (Sects. M3.3.3 and 3 contain the related theory). The spectra are shown in Fig. M5(a) and we mention that they have been directly used to obtain also the non-linear plot of Fig. 3 (the black lines with circles there). Hence the red and black plots of Fig. 3 were done at the linear-response and the ITER1 theory levels, respectively.

The ITER2 curves in Fig. 4 (the green lines) employ the first correction to include the impact of the non-equilibrium electrochemical potentials according to the iterative scheme of Sect. M3.3.4. We see that the impact of the non-equilibrium conditions is noticeable and accurate solutions of the model under study can not neglect them. It is even much clearly seen from the comparison of the differential conductances in panes (b), (c), (e) and (f) of Fig. M6. In terms of the currents the results seem to be converged at the ITER2 level. This is seen when at least a subset of ITER3 results is shown (the blue circles). Complete results for the currents at the ITER3 level are provided in Fig. M6. Although we have available also a subset of the ITER4 results for the currents, we do not show it as it would be indistinguishable from the ITER3 currents. As can be seen from Fig. M6, the derivatives of the currents (the differential conductances) converged at the ITER3 level, i. e. the currents and the electrochemical potentials became self-consistent. Although the potentials themselves may be of secondary interest, we provide results for them in Fig. 5.

# References


[1] M. Büttiker, Phys. Rev. Lett. **57**, 1761 (1986).

[2] K. Nakada, M. Fujita, G. Dresselhaus, M.S. Dresselhaus, Phys. Rev. B **54**, 17954 (1996).

[3] Y.-W. Son, M.L. Cohen, S.G. Louie, Phys. Rev. Lett. **97**, 216803 (2006).

[4] S. Wang, L. Talirz, C.A. Pignedoli, X. Feng, K. Müllen, R. Fasel, P. Ruffieux, Nature Commun. **7**, 11507 (2016).
